# Supplementary material for: Dark Z at the International Linear Collider
Source: arXiv:2205.10304 source file (2022-06-28)
Supplement: Supplementary file 1 [file FlipAdditionalHeader.tex]

%!TEX root = paper.tex
%% Update the above with the appropriate root

%% Place additional project-specific macros, package calls here
%% These are called before FlipPreambleEnd.tex so that,
%% for example, they are called before hyperref

%% Example: replace YourName with your name
\newcommand{\YourName}[1]{{	
	\color{blue!50!black}\footnotesize
	[\textbf{\textsf{YourName}}: \textsf{#1}]}}
